# Supplementary material for: Demystifying Privacy Policy of Third-Party Libraries in Mobile Apps
Source: arXiv:2301.12348 source file (2023-09-09)
Supplement: Supplementary file 1 [file Appendix.tex]

% \section{App's Privacy Policy}

% \subsection{Data Usage in a Table}
% \textbf{com.spotify.tv.android}
% it's privacy policy:
% \begin{figure}
%     \centering
%     \includegraphics[width=0.5\textwidth]{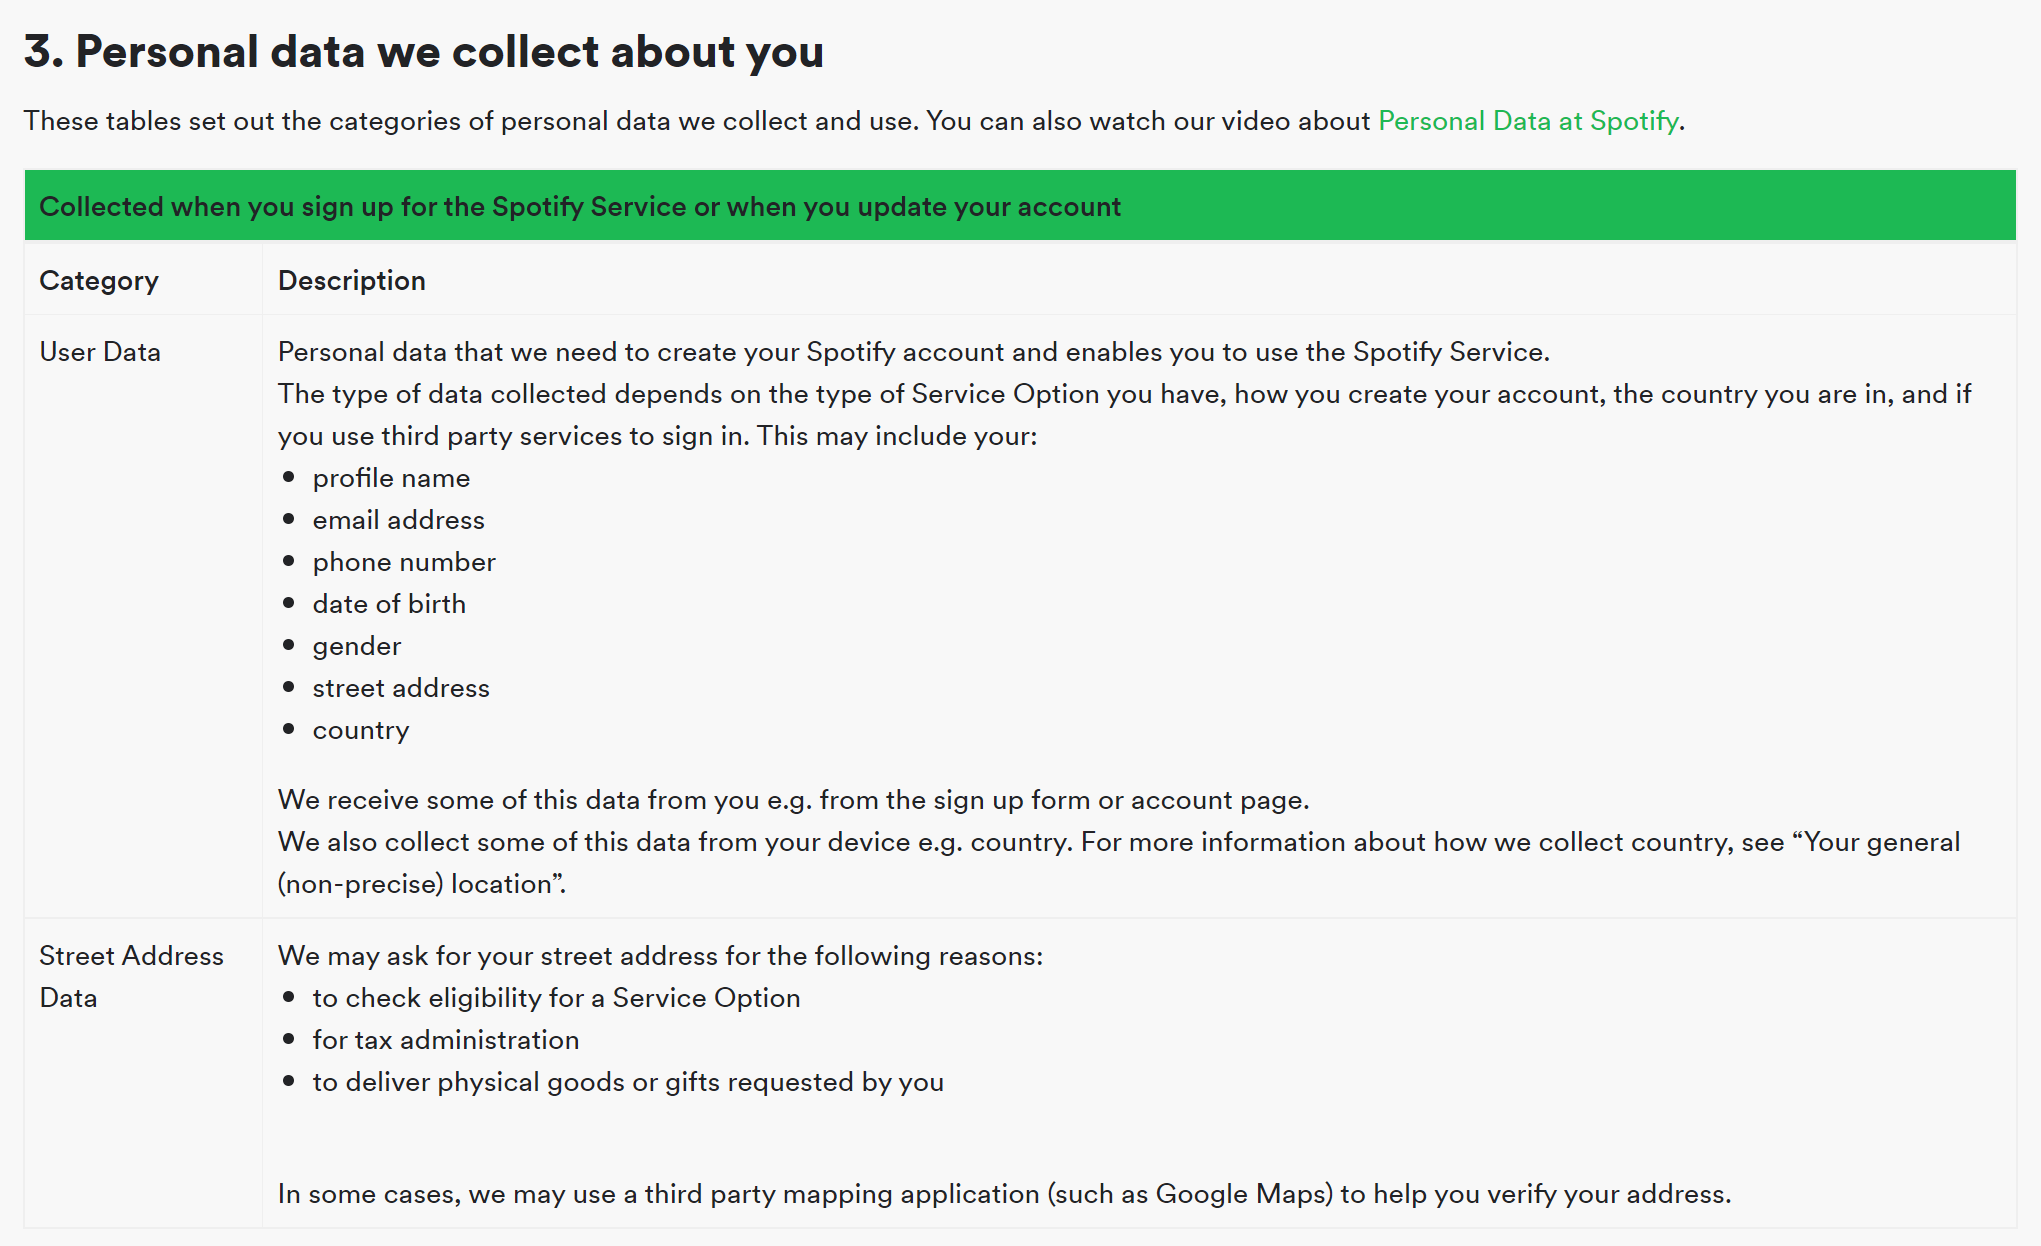}
%     \caption{Data usage in privacy policy of com.spotify.tv}
%     \label{fig:pp_table}
% \end{figure}

% \subsection{Data Sharing with Enumeration}
% \label{app:demo:tpl_enumeration}
% \begin{figure}
%     \centering
%     \includegraphics[width=0.5\textwidth]{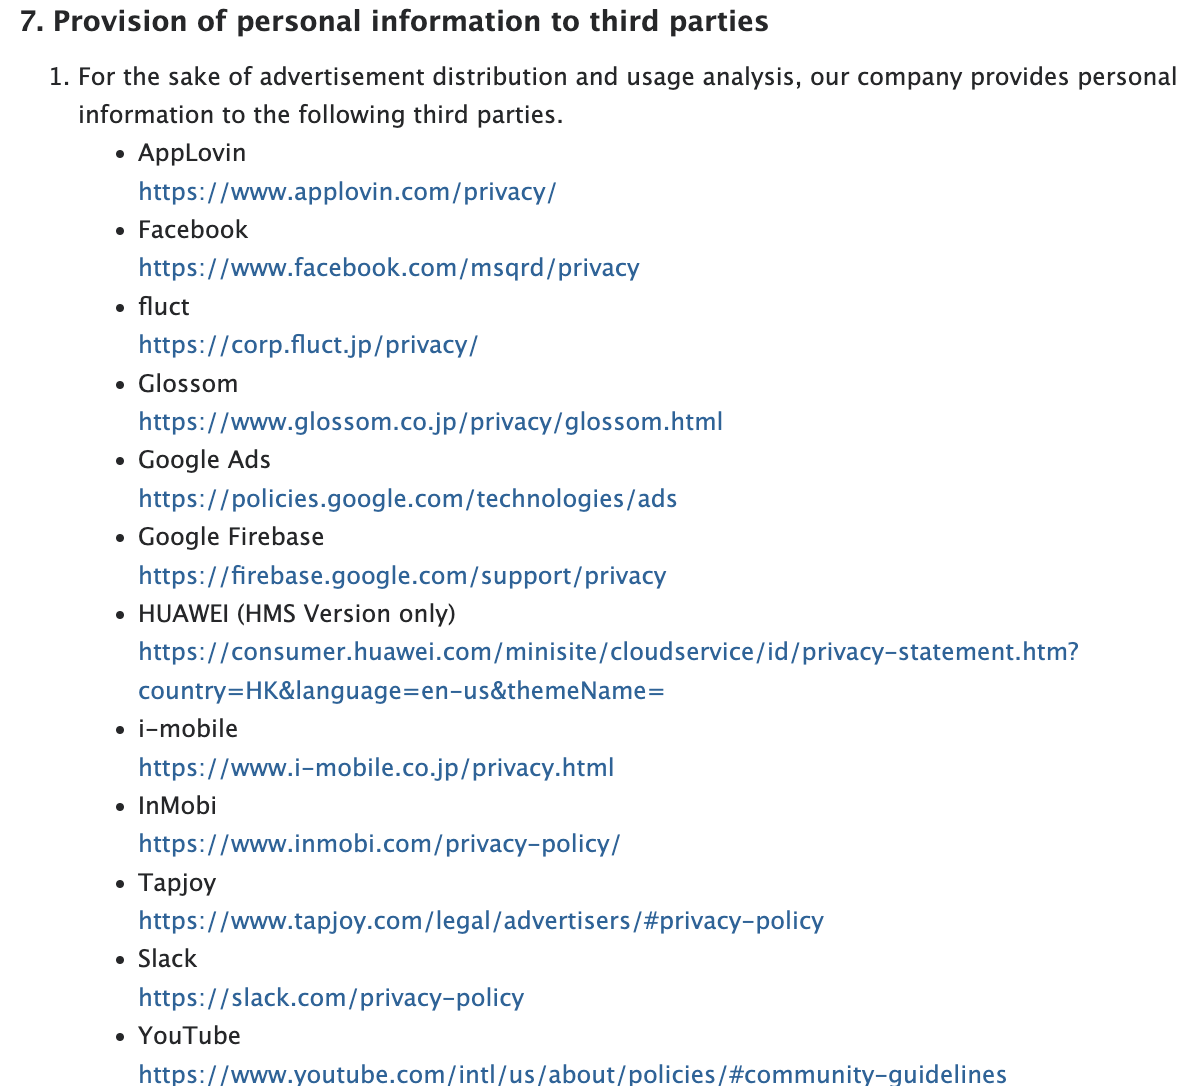}
%     \caption{TPL usage in privacy policy of jp.ne.ibis.ibispaintx.app}
%     \label{fig:pp_tpl_list}
% \end{figure}

\section{Regulations requirements}
\subsection{Information security technology—Personal information (PI) security specification -- China} 
\begin{itemize}

\item 5.5. 4) Purposes of the sharing, transfer and public disclosure of PI, the types of PI
involved, the types of third parties receiving the PI, and respective security and
legal responsibilities;

\item 8.3. b) If a PI Controller has shared PI with, or transferred PI to a third party in violation of laws or regulations, or in violation of its agreement with the PI Subject, and the PI Subject requests deletion, the PI Con troll er shall immediately stop the sharing and transfer, and notify the third p arty to delete the information in a timely manner.

\item 9.6. a) If a PI Controller and a third party are common controllers of PI, the PI Controller shall, through contracts or other means, jointly determine with the third party the PI security requirements to be met, clarify their respective responsibilities and obligations, and inform PI Subjects clearly;
b) If a PI Controller fails to explicitly inform the PI Subjects of the identity of the third party and the PI security responsibilities and obligations borne by the PI Controller and the third party respectively, the PI Controller shall bear the responsibility for any PI security incident caused by the third party.
Note 1: If the PI Controller deployed a third-party plugin to collect PI during the delivery of a product or service (for example, a website operator deploys statistical analysis tools, software development kits (SDKs), or map APIs on its web pages or in its applications) and the third-party did not separately obtain consent from the PI Subjects for collecting their PI, then the PI Controller and the third party are common controllers of PI during the PI collection period.

\item 9.7. h) In the case where a product or service is embedded with or connected to a third party automation tool (such as code, script, interface, algorithm model, software development kit, and mini program), the following measures should be taken: 1) Conduct technical testing to ensure that the collection and use of PI meets the agreed requirements; 2) Audit the collection of PI by the automation tool embedded or connected by the third party and cut off its access in time upon discovery of any behavior beyond the agreed scope.

\end{itemize}

\subsection{Cybersecurity Practices Guidelines – Security Guidelines for Using Software Development Kit (SDK) for Mobile Internet Applications (App) (TC260-PG-20205A) -- CHINA}

(Only Chinese version provided) 

English url \url{https://ca.practicallaw.thomsonreuters.com/w-020-9089?transitionType=Default&contextData=(sc.Default)&firstPage=true}

%\begin{itemize}
 %   \item 3) 行为安全性评估，包括但不限于:调用的敏感权限、目的和频率;收集的个人信息类型、目的和频率;个人信息回传服 务器域名、IP地址、所在地域;是否存在热更新行为及热更 新是否可主动关闭;传输数据是否加密;是否存在单独收集 用户个人信息的界面;是否存在后台自启动和关联启动后收 集个人信息的行为等。
%\end{itemize}

\subsection{General Data Protection Regulation (GDPR) -- EU}

\begin{itemize}
    \item (47) The legitimate interests of a controller, including those of a controller to which the personal data may be disclosed, or of a third party, may provide a legal basis for processing, provided that the interests or the fundamental rights and freedoms of the data subject are not overriding, taking into consideration the reasonable expectations of data subjects based on their relationship with the controller.
    
    \item Article 4 definition. (69) Where personal data might lawfully be processed because processing is necessary for the performance of a task carried out in the public interest or in the exercise of official authority vested in the controller, or on grounds of the legitimate interests of a controller or a third party, a data subject should, nevertheless, be entitled to object to the processing of any personal data relating to his or her particular situation. It should be for the controller to demonstrate that its compelling legitimate interest overrides the interests or the fundamental rights and freedoms of the data subject
    
    \item Article 6 1 (f) processing is necessary for the purposes of the legitimate interests pursued by the controller or by a third party, except where such interests are overridden by the interests or fundamental rights and freedoms of the data subject which require protection of personal data, in particular where the data subject is a child.
\end{itemize}

\subsection{Children’s Online Privacy Protection Act (COPPA)}
\begin{itemize}
    \item 5 However, under the sliding scale approach, operators that keep children’s information internal and do not disclose it publicly or to third parties also can obtain parental consent by a less costly method, i.e., by email with a follow-up contact with the parent to confirm the consent.
    
    \item 5 Most commenters responding to the January 2005 NPR and the April 2005 FRN agreed that more secure electronic mechanisms and infomediary services for obtaining verifiable parental consent still were not widely available at a reasonable cost.66 Similarly, most commenters agreed that disclosures of children’s personal information to third parties or publicly, such as in a chatroom or on a social networking site, continued to pose greater risks to children’s safety and privacy than when an operator keeps the information internal
\end{itemize}

\subsection{California Consumer Privacy Act (CCPA) -- California}
\begin{itemize}
    \item  privacy policy should disclose the categories of third-parties with whom the business shared personal information
\end{itemize}
